# Supplementary material for: Observation of the Schmid-Bulgadaev dissipative quantum phase transition
Source: arXiv:2304.05806 ancillary file (2023-04-12)
Supplement: Supplementary file 1 [file Supplementary_Materials.pdf]

# Supplementary Materials for

## Observation of Schmid-Bulgadaev dissipative quantum phase transition

R. Kuzmin, N. Mehta, N. Grabon, R. Mencia, A. Burshtein, M. Goldstein, and V. E. Manucharyan

Correspondence to: rkuzmin@wisc.edu.

**This PDF file includes:**

Materials and Methods
Theory of the junction effects on the dynamics of its environment
Figs. SF1 to SF6
Table ST1

# S.I. MATERIALS AND METHODS

## A. Device parameters

Table ST1 shows the complete list of the device parameters. To find the waveguides' free spectral ranges $\Delta$ and the cut-off frequencies $\omega_p/2\pi$, we measured the wave dispersion following a previously established procedure [1]. The measurements were done at half-integer flux values through the junction's loop when the junction does not affect the waveguide's standing-wave modes. As in [1], we used two methods to find the impedances $Z/R_Q$, employing either the measured areas of the arrays' junctions or the dimensions of the arrays. Both methods produced similar impedance values. We took their average as the measured impedance value and their difference as the impedance uncertainty.

TABLE ST1. Device parameters

| $Z/R_Q$ | $\omega_p/2\pi$, GHz | $\Delta$, MHz | $A$, $\mu$m$^2$ | $Z^{\rm fit}/R_Q$ | $E_{\rm J}^{fit}/h$, GHz | $E_{\rm C}^{fit}/h$, GHz | $E_{\rm J}^{fit}/E_{\rm C}^{fit}$ |
|---|---|---|---|---|---|---|---|
| $0.34 \pm 0.03$ | 26.4 | 409 | 0.0128 | 0.39 | 1.4 | 18.3 | 0.08 |
| $0.39 \pm 0.05$ | 23.3 | 347 | 0.0066 | 0.46 | 0.8 | 24.5 | 0.03 |
| $0.84 \pm 0.09$ | 22.5 | 167 | 0.0160 | 0.88 | 1.7 | 12.1 | 0.14 |
| $1.43 \pm 0.03$ | 26.1 | 172 | 0.0103 | 1.39 | 1.3 | 13.5 | 0.10 |
| $2.92 \pm 0.02$ | 19.0 | 104 | 0.0262 | 2.91 | 3.7 | 8.9 | 0.42 |
| $3.01 \pm 0.04$ | 18.4 | 102 | 0.0374 | 3.05 | 5.2 | 8.8 | 0.59 |

## B. Measurement of a phase shift in a single device at varying impedance

The phase shift, which a Josephson junction induces on a waveguide's standing-wave mode $k$, can be defined as $\delta_k = \pi(f_k(IFQ) - f_k(HFQ))/\Delta$, where $\Delta = v/2L$ is the free spectral range of the waveguide defined by its length $L$ and wave velocity $v$. $f_k(IFQ) - f_k(HFQ)$ is the difference in the mode's frequency at integer and half-integer dimensionless flux $\Phi/\Phi_0$. This frequency difference might be quite small and become obscured under large impedance variation, as the frequencies of all the standing-wave modes experience a significant shift (see Fig. SF1).

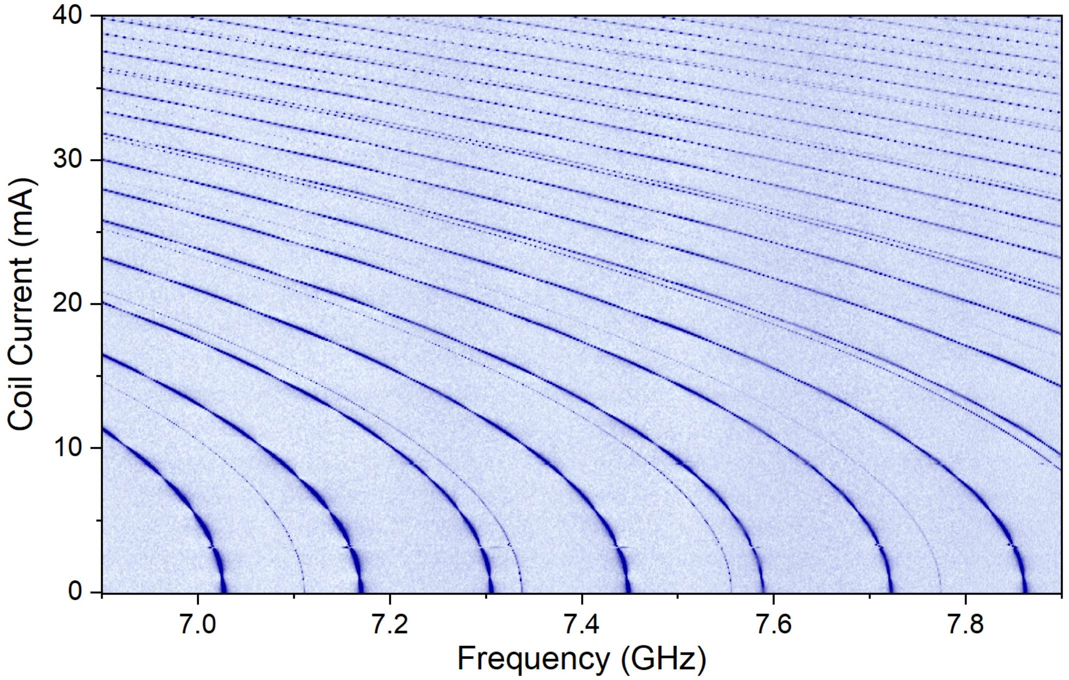


FIG. SF1. An example of the reflection spectroscopy measured on the device with $Z/R_Q \approx 0.84$ at progressively larger perpendicular magnetic fields. The coil current controls the field. The color represents the reflection magnitude and is optimized for the best visibility. Notice the two sets of modes.

For improved measurement accuracy, we employed the fact that the coplanar stripline geometry of our Josephson transmission lines supports two types of standing-wave modes: antisymmetric and symmetric [1]. In the spectroscopy, the former are bright lines with modulation in their linewidth, and the latter are faint narrow lines with larger spacing (Fig. SF1). The antisymmetric modes couple to the Josephson junction and allow us to observe the junction's dynamics. In contrast, the symmetric ones do not interact with the junction, as they create a zero voltage difference at the junction's position. Therefore, we can use symmetric modes as a reference, allowing us to accurately measure the minor variations in the positions of the antisymmetric modes.

We used the following procedure. At each flux value $\Phi$, which controls the small junction's $E_J$ and the environmental impedance, we measured the frequency $f_k$ and the linewidth of an antisymmetric mode along with the frequency of a symmetric mode $f_s$. Then, the phase shift is given by $\delta_k(\Phi) = \pi\beta(\Phi)(f_k(IFQ) - f_k(HFQ))/\Delta(\Phi)$, where $\beta(\Phi) = f_s(0)/f_s(\Phi)$ is the coefficient that compensates the trivial frequency shift induced by the change in the waveguide's free spectral range. Both the impedance and the free spectral range at any flux can be obtained from their values at zero fields using the same coefficient: $Z(\Phi) = \beta(\Phi)Z(0)$, $\Delta(\Phi) = \Delta(0)/\beta(\Phi)$.

## S.II. THEORY OF THE JUNCTION EFFECTS ON THE DYNAMICS OF ITS ENVIRONMENT

In this section, we will derive the inelastic decay rates and elastic mode shifts of the array modes, starting from the circuit model. We will consider both a perturbative approach, applicable for frequencies above an emergent RG energy scale, as well as exact solutions at the special points $z = 1$ and $z = 1/2$, which apply at any frequency well below the cutoff, and hence shed light on the low-energy properties of the system.

The circuit Lagrangian describes a SQUID galvanically-coupled to a high-impedance transmission line. We separate the quadratic part from the cosine potential of the SQUID, writing $L = L_0 + L_I$, where

$$L_0 = \frac{\hbar v}{4\pi z}\int_0^l \mathrm{d}x \left[\frac{1}{v^2}(\partial_t\varphi)^2 - (\partial_x\varphi)^2 + \frac{1}{\omega_p^2}(\partial_t\partial_x\varphi)^2\right] + \frac{\hbar^2}{16E_C}(\partial_t\varphi(x=0,t))^2, \quad L_I = E_J(\Phi)\cos(\varphi(x=0,t)). \tag{S1}$$

Here $\varphi(x,t)$ is the superconducting phase field, $v$ is the wave velocity, $\omega_p$ is the plasma frequency, and $z = Z/R_Q$ is the wave impedance normalized by the superconducting resistance quantum, $R_Q = 2\pi\hbar/(2e)^2$. For brevity, in the following we omit the explicit $\Phi$ dependence of $E_J$. We assume throughout that $E_J/E_C \ll 1$.

### A. The linear limit

To lowest order in $E_J/E_C$, one may discard the cosine term $L_I$. The remaining Lagrangian is quadratic and is diagonalized by plane waves, $\varphi_k(x,t) = \sin(kx+\delta_k)e^{-i\omega_k t}$. Assuming $\omega_p \ll v$, the dispersion relation is given by $\omega_k = vk/\sqrt{1+(vk/\omega_p^2)}$. The phase shift of the plane waves, $\delta_k$, results from coupling to the SQUID, and is given by $\tan\delta_k = -\sqrt{\omega_p^2-\omega_k^2}/(\omega_p\omega_k/\Gamma_0)$, where $\Gamma_0 = 1/(ZC) = 4E_C/(\pi z\hbar)$ is the inverse $ZC$ time of the line and the SQUID. The termination of the line at the other end, $x = l$, may be approximated as an open port, leading to the boundary condition $\partial_x\varphi(x=l,t) = 0$, and hence to the quantization of the mode frequencies, $kl + \delta_k = \pi m$ with $m \in \mathbb{N}$. The mode spacing is then approximated by $\Delta_k = \Delta(1-(\omega_k/\omega_p)^2)^{3/2}$, with $\Delta = \pi v/l$. The modes obey an orthogonality relation,

$$\frac{2e^2}{\pi z\hbar v}\int_0^l \mathrm{d}x\varphi_k^*(x,t)\varphi_{k'}(x,t) + \frac{2e^2 v}{\pi\hbar z\omega_p^2}\int_0^l \mathrm{d}x\partial_x\varphi_k^*(x,t)\partial_x\varphi_{k'}(x,t) + \frac{e^2}{2E_C}\varphi_k^*(0,t)\varphi_{k'}(0,t) = C_k\delta_{k,k'}, \tag{S2}$$

where $\delta_{k,k'}$ is the Kronecker delta (not to be confused with the phase shift), and the capacitance of mode $k$ is $C_k = e^2 l/(\pi z\hbar v) \times 1/(1-(\omega_k/\omega_p)^2)$.

We proceed to quantize the field by introducing bosonic mode creation and annihilation operators, $a_k^\dagger$ and $a_k$, respectively, obeying bosonic commutation relations, $[a_k, a_{k'}^\dagger] = \delta_{k,k'}$, etc. The quadratic Hamiltonian assumes a diagonal form, $H_0 = \sum_k \hbar\omega_k a_k^\dagger a_k$, and the field operator $\varphi(x,t)$ becomes

$$\varphi(x,t) = \sum_k \sin(kx+\delta_k)\varphi_k(t), \qquad \varphi_k(t) = \sqrt{\frac{2z\Delta_k}{\omega_k}}\frac{1}{(1-(\omega_k/\omega_p)^2)^{1/4}}\left(a_k e^{-i\omega_k t} + a_k^\dagger e^{i\omega_k t}\right). \tag{S3}$$

## B. Perturbative calculation of the inelastic decay rate and elastic mode shift

In this subsection, we treat the cosine term, $L_I = E_J \cos(\varphi(x=0,t))$, as a perturbation, and perform a diagrammatic expansion to calculate the photon propagator. This propagator admits a self-energy, which yields the elastic mode shift $\delta\omega_k$ and inelastic decay rate $\Gamma_k^{\text{in}}$.

Using the creation and annihilation operators $a_k, a_k^\dagger$, the perturbation Hamiltonian $H_I = -E_J \cos(\varphi(x=0,t))$ assumes the form

$$H_I = -E_J \cos\left(\sum_k f_k \left(a_k e^{-i\omega_k t} + a_k^\dagger e^{i\omega_k t}\right)\right), \quad f_k^2 = \frac{2z\Delta_k}{\omega_k} \frac{\sqrt{1-(\omega_k/\omega_p)^2}}{1+((\omega_p/\Gamma_0)^2-1)(\omega_k/\omega_p)^2}. \tag{S4}$$

The factor $f_k$ sets the coupling strength of each mode to the perturbation term. Note the denominator of $f_k^2$ above, indicating that the cutoff frequency is effectively set by the lower among $\Gamma_0$ and $\omega_p$. Using Eq. (S4), we may calculate the time-ordered photon propagator, $G_k^{\mathcal{T}}(t-t') = -i\langle \mathcal{T}\varphi_k(t)\varphi_k(t')\rangle_H$, where calligraphic $\mathcal{T}$ represents time-ordering (not to be confused with the temperature $T$). Expanding the cosine as a Taylor series allows us to contract the external legs $\varphi_k$ with $H_I$, leading to a diagrammatic expansion which results in $G_k^T(\omega) = 1/(\omega^2 - (\omega_k - \Sigma_k^T(\omega))^2)$, where $\Sigma_k^T(\omega)$ is the time-ordered self-energy. The leading terms in the self-energy are the following:

$$\Sigma_k^{\mathcal{T}}(t-t') = \tag{S5}$$

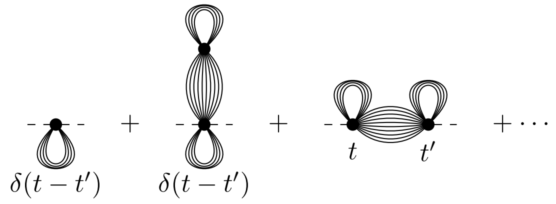


The dashed lines represent the external legs of the self-energy, which are contracted to the $\varphi_k$ legs or to each other (at different intermediate times) in the calculation of $G_k^{\mathcal{T}}(\omega)$. The first term in Eq. (S5) involves a single copy of $H_I$. In the diagrammatic expansion of the propagator, this term corresponds to two external $\varphi(x=0,t)$ legs that are pulled out of the cosine, and the remaining legs are contracted with each other at equal times, $t=t'$, represented by the closed loops. This term is of order $E_J$, and is given by $\langle E_J \cos(\varphi(x=0,t))\rangle_{H_0}$; however, it vanishes in the thermodynamic limit as a power law in the system size $l$. The second term is very similar to the first one, and yields the leading contribution to the cosine average, $\langle E_J \cos(\varphi(x=0,t))\rangle_H$:

$$\langle E_J \cos(\varphi(x=0,t))\rangle_H = \frac{iE_J^2}{\hbar}\int \mathrm{d}t_1 \, \langle \mathcal{T} \cos(\varphi(x=0,t)) \cos(\varphi(x=0,t_1))\rangle_{H_0}. \tag{S6}$$

It involves contractions between two copies of the cosine at equal times, as well as contractions within each cosine. The third term in Eq. (S5) involves two copies of $H_I$ at different times, $t, t'$; a single external $\varphi(x=0,t^{(\prime)})$ leg is pulled out of each cosine, and the remaining legs are contracted among themselves. This gives rise to the time-ordered sine-sine correlator, $\Pi^{\mathcal{T}}(t_1-t_2) = 2i\,\langle \mathcal{T}\sin(\varphi(x=0,t_1)\sin(\varphi(x=0,t_2)\rangle_{H_0}$, whose Fourier transform is given by

$$\Pi^{\mathcal{T}}(\omega) = 2i\int_0^\infty \mathrm{d}t \cos(\omega t) \exp\left\{-\sum_k f_k^2 \left[\left(1-e^{-i\omega_k|t|}\right)(1+n_B(\omega_k)) + \left(1-e^{i\omega_k|t|}\right) n_B(\omega_k)\right]\right\}, \tag{S7}$$

where $n_B(\omega_k)$ is the Bose-Einstein distribution, $n_B(\omega_k) = 1/(e^{\hbar\omega_k/(k_B T)}-1)$. In order to evaluate $\Pi^{\mathcal{T}}(\omega)$ numerically, we use the fact that in the thermodynamic limit, summations over $k$ may be replaced by frequency integrals, $\sum_k \to \int_0^{\omega_p} d\omega_k/\Delta_k$. Note that both the second and third terms in Eq. (S5) are of second order in $E_J^2$. Moreover, it is evident from Eq. (S5) that the cosine average is related to the sine-sine correlator; namely, $\langle E_J \cos(\varphi(x=0,t_1))\rangle_H = \frac{E_J^2}{2\hbar}\Pi^{\mathcal{T}}(\omega=0)$. Putting the pieces together, we arrive at the retarded self-energy,

$$\Sigma_k^{\mathcal{R}}(\omega) = (E_J/\hbar)^2 f_k^2 \left(\Pi^{\mathcal{R}}(\omega) - \Re\Pi^{\mathcal{R}}(\omega=0)\right), \tag{S8}$$

whose real and imaginary parts, evaluated at $\omega=\omega_k$, correspond to the elastic mode shift and inelastic decay rate of the mode $k$, respectively:

$$\delta\omega_k = \Re\Sigma_k^{\mathcal{R}}(\omega_k), \quad \Gamma_k^{\text{in}}/2 = \Im\Sigma_k^{\mathcal{R}}(\omega_k). \tag{S9}$$

Here $\Pi^{\mathcal{R}}(\omega)$ is the retarded sine-sine correlator, related to the time-ordered correlator through $\Pi^{\mathcal{R}}(\omega) = \Re\Pi^{\mathcal{T}}(\omega) + i\tanh(\hbar\omega/(2k_BT))\Im\Pi^{\mathcal{T}}(\omega)$.

In the limit $\omega_p \gg \Gamma_0$, the correlator $\Pi^{\mathcal{R}}(\omega)$ may be expressed in terms of exponential and hypergeometric functions at both zero and finite temperatures. One may then obtain asymptotic expansions for $\Gamma_k^{\text{in}}$ and $\delta\omega_k$. First, consider $\Gamma_k^{\text{in}}$:

$$\Gamma_k^{\text{in}}/2 \approx \begin{cases} \frac{\Delta\pi z\Gamma^2(z)}{\Gamma(2z)}\left(\frac{E_J/\hbar}{\pi\Gamma_0/2}\right)^2\left(\frac{4k_BT}{\hbar\Gamma_0}\right)^{2z-2}, & \omega \ll k_BT/\hbar \ll \Gamma_0, \\ \frac{\Delta\pi z}{\Gamma(2z)}\left(\frac{E_J/\hbar}{\pi\Gamma_0/2}\right)^2\left(\frac{\omega}{\pi\Gamma_0/2}\right)^{2z-2}, & k_BT/\hbar \ll \omega \ll \Gamma_0, \\ \frac{\Delta\pi z}{\Gamma(2z)}\left(\frac{E_J/\hbar}{\pi\Gamma_0/2}\right)^2\left(\frac{\omega}{\pi\Gamma_0/2}\right)^{2z-4} e^{-\omega/(\pi\Gamma_0/2)}, & k_BT/\hbar \ll \Gamma_0 \ll \omega, \end{cases} \tag{S10}$$

where $\Gamma(x)$ is the gamma function [2]. The diverging power law of $\Gamma_k^{\text{in}}$ for $z < 1$ and $\omega \ll \Gamma_0$ implies that the cosine is relevant for such impedances, giving rise to an emergent RG energy scale [3], $E_J^*/\hbar = ((E_J/\hbar)/\Lambda^z)^{1/(1-z)}$, where $\Lambda$ is a cutoff frequency roughly set by $\Lambda = \min\{\omega_p, \Gamma_0\}$. Perturbation theory fails when both the temperature and the frequency are below this scale, $k_BT, \hbar\omega \ll E_J^*$. Since the cosine is relevant for $z < 1$, at low energies the phase $\varphi(x = 0, t)$ is localized around one of its minima, corresponding to a superconducting state. Hence, Eq. (S10) is valid only for large enough frequency or temperature, $\max\{k_BT, \hbar\omega\} \gg E_J^*$. On the contrary, the cosine is irrelevant for $z > 1$, and the perturbative result above applies for arbitrarily small frequency and temperature as long as $E_J/E_C$ is small enough. In that case, $\varphi(x = 0, t)$ is free to fluctuate at low energies, corresponding to an insulating state.

Asymptotic expansions for $\delta\omega_k$ are also useful for comparison with the experiment. First, for low frequencies, $\omega \ll k_BT/\hbar \ll \Gamma_0$:

$$\delta\omega_k\left(\omega \ll k_BT/\hbar \ll \Gamma_0\right) = \begin{cases} -\dfrac{4\Delta z\tan\left(\pi z\right)C\left(z\right)\Gamma^2\left(z\right)}{\Gamma\left(2z\right)}\left(\frac{E_J/\hbar}{\pi\Gamma_0/2}\right)^2\left(\frac{4k_BT/\hbar}{\Gamma_0}\right)^{2z-3}\frac{\omega}{\pi\Gamma_0/2}, & z < 3/2 \text{ and } z \neq 1/2, 1, \\ 7\Delta\zeta\left(3\right)\left(\frac{E_J/\hbar}{\pi\Gamma_0/2}\right)^2\left(\frac{4k_BT/\hbar}{\Gamma_0}\right)^{-2}\frac{\omega}{\pi\Gamma_0/2}, & z = 1/2, \\ 2\Delta\left(\frac{E_J/\hbar}{\pi\Gamma_0/2}\right)^2\left(1 - \log\left(\frac{4k_BT/\hbar}{\Gamma_0}\right)\right)\frac{\omega}{\pi\Gamma_0/2}, & z = 1, \\ \frac{3\Delta}{2}\left(\frac{E_J/\hbar}{\pi\Gamma_0/2}\right)^2\left(\log\left(\frac{4k_BT/\hbar}{\Gamma_0}\right) + 0.717\right)\frac{\omega}{\pi\Gamma_0/2} & z = 3/2, \\ \frac{2\Delta z}{(1-2z)(2-2z)(3-2z)}\left(\frac{E_J/\hbar}{\pi\Gamma_0/2}\right)^2\frac{\omega}{\pi\Gamma_0/2}, & z > 3/2, \end{cases} \tag{S11}$$

where

$$C\left(z\right) = \frac{z\left[\psi\left(1+z\right) - \psi\left(1-z\right)\right]\left[2 + z\psi\left(1-z\right) - z\psi\left(1+z\right)\right] + z^2\left[\psi'\left(1-z\right) - \psi'\left(1+z\right)\right] - 2}{8z^2}, \tag{S12}$$

and $\psi(x)$ and $\zeta(x)$ are, respectively, the digamma and zeta functions [2]. Next, for frequencies above the temperature and below the elastic decay rate, $k_BT/\hbar \ll \omega \ll \Gamma_0$:

$$\delta\omega_k\left(k_BT/\hbar \ll \omega \ll \Gamma_0\right) = \begin{cases} \frac{\pi\Delta z\tan(\pi z)}{\Gamma(2z)}\left(\frac{E_J/\hbar}{\pi\Gamma_0/2}\right)^2\left[\frac{\Gamma^2(z)}{\pi}\left(\frac{4k_BT/\hbar}{\Gamma_0}\right)^{2z-1}\frac{\pi\Gamma_0/2}{\omega} - \left(\frac{\omega}{\pi\Gamma_0/2}\right)^{2z-2}\right], & z < 1/2, \\ \Delta\left(\frac{E_J}{\pi\Gamma_0/2}\right)^2\left[\log\left(\frac{\omega}{\pi\Gamma_0/2}\right) - 2\log\left(\frac{E_J}{\pi\Gamma_0/2}\right) - \log\pi\right]\frac{\pi\Gamma_0/2}{\omega}, & z = 1/2, \\ -\frac{\pi\Delta z\tan(\pi z)}{\Gamma(2z)}\left(\frac{E_J/\hbar}{\pi\Gamma_0/2}\right)^2\left(\frac{\omega}{\pi\Gamma_0/2}\right)^{2z-2}, & 1/2 < z < 3/2 \text{ and } z \neq 1, \\ -\Delta\left(1 - 2\psi\left(2\right) + 2\log\left(\frac{\omega}{\pi\Gamma_0/2}\right)\right)\left(\frac{E_J/\hbar}{\pi\Gamma_0/2}\right)^2\frac{\omega}{\pi\Gamma_0/2}, & z = 1, \\ -\frac{3\Delta}{2}\left(-\frac{3}{2} + \psi\left(3\right) - \log\left(\frac{\omega}{\pi\Gamma_0/2}\right)\right)\left(\frac{E_J/\hbar}{\pi\Gamma_0/2}\right)^2\frac{\omega}{\pi\Gamma_0/2}, & z = 3/2, \\ \frac{2\Delta z}{(1-2z)(2-2z)(3-2z)}\left(\frac{E_J/\hbar}{\pi\Gamma_0/2}\right)^2\frac{\omega}{\pi\Gamma_0/2}, & z > 3/2. \end{cases} \tag{S13}$$

Finally, for frequencies above the elastic decay rate, $k_BT/\hbar \ll \Gamma_0 \ll \omega$:

$$\delta\omega_k(k_BT/\hbar \ll \Gamma_0 \ll \omega) \approx -4\Delta z^2\left(\frac{E_J/\hbar}{\pi\Gamma_0/2}\right)^2\left(\frac{\omega}{\pi\Gamma_0/2}\right)^{-5}. \tag{S14}$$

The inelastic decay rate and elastic mode shifts for several values of the normalized impedance $z$ are displayed

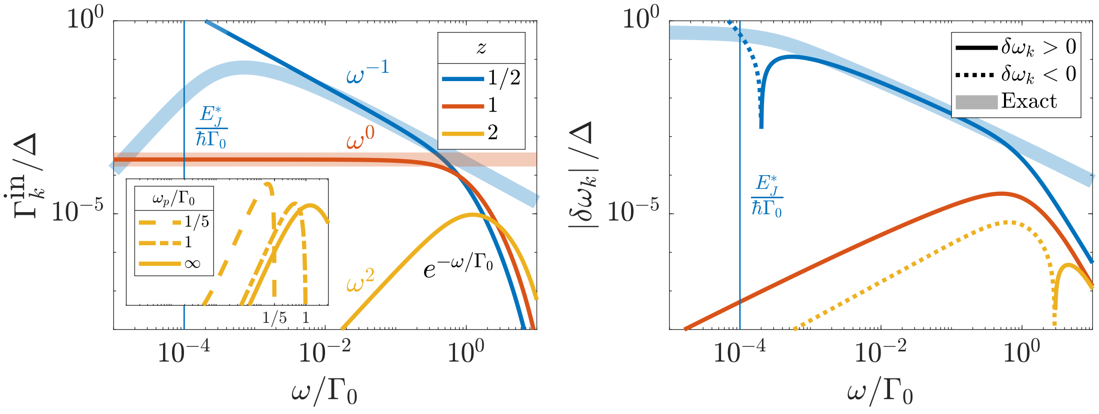


FIG. SF2. Frequency dependence of the inelastic decay rate (left) and elastic mode shift (right) for $(E_J/\hbar)/\Gamma_0 = 0.01$, $\omega_p = \infty$ and $T = 0$, evaluated using the perturbative solution (thin lines) in Eq. (S9), as well as the exact solutions available for $z = 1/2$ and $z = 1$, obtained from the reflection coefficients in Eqs. (S24) and (S29), respectively (wide shaded lines). The exact solutions apply for all frequencies well below the cutoff, $\omega \ll \Gamma_0$, while perturbation theory applies above the renormalization-group generated scale $E_J^*/\hbar$ (marked by thin blue vertical lines for $z = 1/2$; note that $E_J^* = ((E_J/\hbar)/\Gamma_0^z)^{1/(1-z)}$ vanishes for $z \to 1$). Both agree over the overlap of these two regimes, $E_J^*/\hbar \ll \omega \ll \Gamma_0$, except for the mode shift at $z = 1$, which vanishes in the exact solution and is thus dominated by finite-cutoff corrections for all frequencies. The inset shows the inelastic decay rate for $z = 2$ and several values of $\omega_p$ (same axes as main figure; the values of $\omega_p/\Gamma_0$ are indicated on the horizontal axis.)

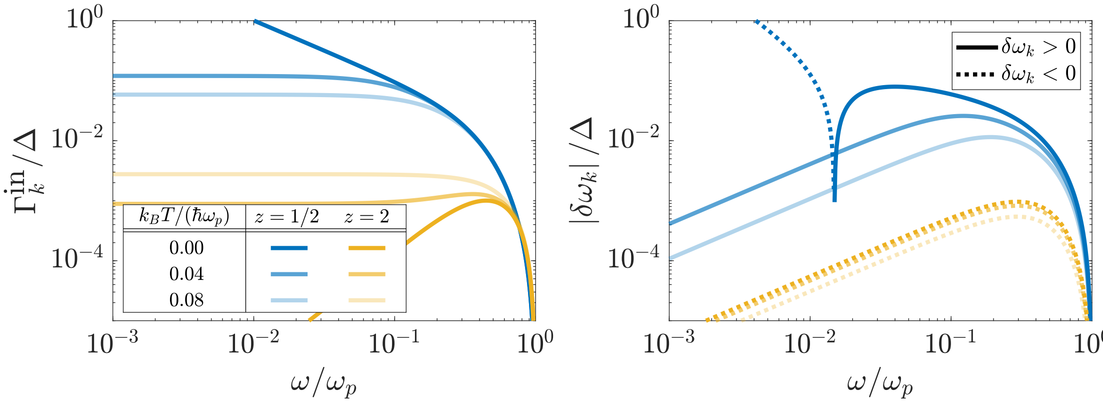


FIG. SF3. Frequency dependence of the inelastic decay rate (left) and elastic mode shift (right) for $(E_J/\hbar)/\omega_p = 0.05$, $\Gamma_0/\omega_p = 1/2$, and several temperatures $T$, evaluated using the perturbative solution in Eq. (S9). At large enough $T$ and $z$, the slope of $\Gamma_k^{\mathrm{in}}$ changes sign.

in Fig. SF2. Temperature dependence is depicted in Fig. SF3; one may note that for large $z$, as temperature increases, the slope of the decay rate flattens out and even changes sign.

This concludes the perturbative solution of $\Gamma_k^{\mathrm{in}}$ and $\delta\omega_k$, which, as mentioned above, holds only for $\max\{k_BT, \hbar\omega\} \gg E_J^*$. In the following subsection, we obtain an exact solution for $\Gamma_k^{\mathrm{in}}$ and $\delta\omega_k$ at $z = 1/2$, applicable both below and above $E_J^*$.

### C. Exact solution for $z = 1/2$

Consider the Lagrangian in Eq. (S1) with $z = 1/2$, $\omega_p \to \infty$, and the scaling limit $E_J, E_C \to \infty$, such that $\Gamma_0 \to \infty$ while $E_J^* \sim E_J^2/E_C$ remains finite:

$$L = \frac{\hbar v}{2\pi} \int_0^l \mathrm{d}x \left[ \frac{1}{v^2} (\partial_t \varphi)^2 - (\partial_x \varphi)^2 \right] + E_J \cos(\varphi(x = 0, t)). \tag{S15}$$

The corresponding Hamiltonian is

$$H = \frac{\hbar v}{2\pi} \int_0^l \mathrm{d}x \left[(\pi\rho)^2 + (\partial_x \varphi)^2\right] - E_J \cos(\varphi(x=0,t)), \tag{S16}$$

where $\rho$ is the conjugate momentum field to the field $\varphi$. In this subsection we follow the steps of [3] and obtain an exact solution for the Hamiltonian by introducing a fermionic field proportional to the exponent of the bosonic field, $\Psi(x) \sim e^{i\varphi(x)}$.

The cosine term poses technical difficulties in straightforward refermionization, as it would lead to terms in the Hamiltonian that are linear in $\Psi(x=0)$ and $\Psi^\dagger(x=0)$. To overcome this problem, one may introduce a spin operator in front of the cosine term, $E_J \cos(\varphi(x=0,t)) \to S_x E_J \cos(\varphi(x=0,t))$, so that the new Hamiltonian commutes with $S_x$ and is therefore equivalent to the original Hamiltonian for either $S_x = 1$ or $S_x = -1$ (in the latter case, up to a shift of $\varphi$). Writing the spin operator in terms of a fermionic creation operator $d^\dagger$, namely $S_x = S_+ + S_- = d^\dagger + d$, the fermionic field $\Psi(x)$ is defined as (up to Klein factors, which are not important in the following [3])

$$\Psi(x) = \frac{1}{\sqrt{2\pi a_0}} e^{i\pi d^\dagger d} e^{i\varphi(x)}, \tag{S17}$$

where $a_0$ is a short distance cutoff, whose specific value will be determined later. The factor $e^{i\pi d^\dagger d}$ ensures that the operators $\Psi(x)$ and $d$ anticommute. Introducing the eigenmodes of the fermionic operators, $\Psi(x) = 1/\sqrt{2l}\sum_q \Psi_q e^{iqx}$, we find a Hamiltonian quadratic in $\Psi$ and $d$,

$$H = \sum_q \hbar v q \Psi_q^\dagger \Psi_q - \frac{E_J\sqrt{2\pi a_0}}{2\sqrt{2l}} (d^\dagger - d) \sum_q \left(\Psi_q + \Psi_q^\dagger\right). \tag{S18}$$

We proceed by introducing the current operator, defined by the time derivative of the total charge,

$$Q = e\int_0^l \mathrm{d}x \Psi^\dagger(x)\Psi(x) = e\sum_q \Psi_q^\dagger \Psi_q,$$
$$J = \partial_t Q = -\frac{i}{\hbar}[Q,H] = \frac{ie}{\hbar}(d^\dagger - d)\frac{E_J\sqrt{2\pi a_0}}{2\sqrt{2l}} \sum_q \left(\Psi_q^\dagger - \Psi_q\right) = \frac{eE_J}{\hbar}\sin(\varphi(x=0)), \tag{S19}$$

which can be recognized as the Josephson current through the junction. We are interested in the AC conductance $\mathcal{G}(\omega)$, given by the Kubo formula

$$\mathcal{G}(\omega) = \frac{1}{i\hbar\omega} K^{\mathcal{R}}(\omega), \qquad K^{\mathcal{R}}(t) = -i\theta(t)\left\langle [J(t), J(0)]\right\rangle, \tag{S20}$$

where $\theta(t)$ is the Heaviside step function. The quadratic form of the Hamiltonian in Eq. (S18) allows for an exact solution for the imaginary time-ordered current-current correlator,

$$K^{\mathcal{T}}(i\omega_n) = -\frac{e^2}{2\pi} \times \frac{\gamma}{\hbar}\left[\psi\left(\frac{\gamma + \hbar\omega_n}{2\pi k_B T} + \frac{1}{2}\right) - \psi\left(\frac{\gamma}{2\pi k_B T} + \frac{1}{2}\right)\right], \tag{S21}$$

where $\omega_n$ is a bosonic Matsubara frequency and $\gamma = 2\pi a_0 E_J^2/(\hbar v)$ is an energy scale to be found shortly. The retarded correlator is then obtained by analytic continuation, $K^{\mathcal{R}}(\omega) = K^{\mathcal{T}}(i\omega_n \to \omega)$, leading to

$$\mathcal{G}(\omega) = \mathcal{G}_{1/2} \times \frac{i\gamma}{\hbar\omega}\left[\psi\left(\frac{\gamma - i\hbar\omega}{2\pi k_B T} + \frac{1}{2}\right) - \psi\left(\frac{\gamma}{2\pi k_B T} + \frac{1}{2}\right)\right]. \tag{S22}$$

Note that Eq. (S22) is the backscattered AC conductance and should be zero for a decoupled waveguide ($E_J = 0$); $\mathcal{G}_{1/2} = ze^2/(2\pi\hbar) = e^2/(4\pi\hbar)$ is the non-backscattered conductance for $E_J = 0$ [4]. The backscattered conductance defines a reflection coefficient, $\mathcal{G}/\mathcal{G}_{1/2} = (1-r)/2$, related to the elastic mode shift and inelastic decay rate through $r(\omega_k) = e^{-2\pi i \delta\omega_k/\Delta} e^{-\pi\Gamma_k^{\mathrm{in}}/\Delta}$. At $T = 0$ and $\hbar\omega_k \gg \gamma$, one obtains $\Gamma_k^{\mathrm{in}} \approx \Delta\gamma/(2\hbar\omega_k)$; comparing with the perturbative solution below the cutoff in Eq. (S10), we identify $\gamma = 2E_J^*$, where $E_J^*/\hbar = (E_J/\hbar)^2/\Gamma_0$ is the RG

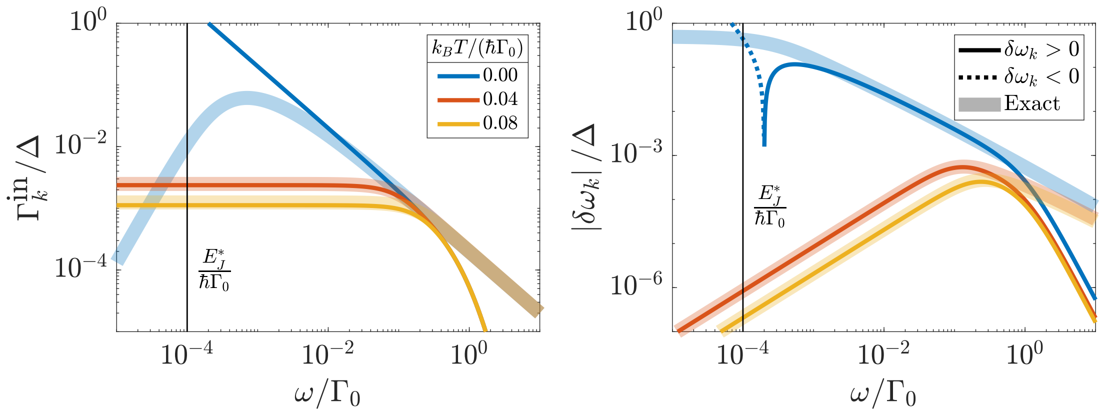


FIG. SF4. Frequency dependence of the inelastic decay rate (left) and elastic mode shift (right) for $z = 1/2$, $\omega_p = \infty$, $(E_J/\hbar)/\Gamma_0 = 0.01$, and several values of $T$. Both the perturbative (thin lines, evaluated using Eq. (S9)) and exact (thick and shaded lines, evaluated from the reflection coefficient in Eq. (S24)) results are displayed. The RG scale $E_J^*$ is depicted by thin black vertical lines. Perturbation theory and the exact results agree in the regime $E_J^*/\hbar \ll \max\{\omega, k_BT/\hbar\} \ll \Gamma_0$.

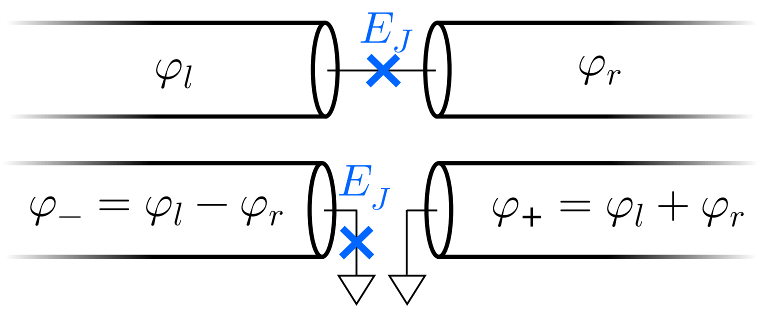


FIG. SF5. Left-right (top) vs. symmetric-antisymmetric (bottom) bases. The former corresponds to Eq. (S25). Only the antisymmetric mode $\varphi_-$ is coupled to the impurity, leading to Eq. (S15).

scale for $z = 1/2$. All in all, the reflection coefficient is given by

$$r(\omega; z = 1/2) = 1 - \frac{4iE_J^*}{\hbar\omega}\left[\psi\left(\frac{2E_J^* - i\hbar\omega}{2\pi k_BT} + \frac{1}{2}\right) - \psi\left(\frac{2E_J^*}{2\pi k_BT} + \frac{1}{2}\right)\right]. \tag{S23}$$

The exact and perturbative inelastic decay rates and elastic mode shifts for several temperatures are displayed in Fig. SF4. We note that the same reflection coefficient may be found by solving a scattering problem for the bosonic operators $a_k, a_k^\dagger$, using the bosonization relation $a_k = \sqrt{\pi/(lk)}\sum_q \Psi_q^\dagger \Psi_{q+k}$ [5].

Let us consider in more details the limit $T = 0$, where the reflection coefficient becomes

$$r(\omega; T = 0; z = 1/2) = 1 - \frac{4iE_J^*}{\hbar\omega}\log\left(1 - \frac{i\hbar\omega}{2E_J^*}\right) \tag{S24}$$

As mentioned above, taking the limit $\hbar\omega \gg E_J^*$ leads to $\Gamma_k^{\rm in} \approx 2\Delta E_J^*/(\hbar\omega) = 2\Delta E_J^2/(\hbar^2\Gamma_0\omega)$, in agreement with Eq. (S10). The mode shift in this limit, $\delta\omega_k \approx 2\Delta E_J^2/(\hbar^2\pi\omega\Gamma_0)\log\left(\hbar^2\omega\Gamma_0/(2E_J^2)\right)$, agrees with the perturbative expansion in Eq. (S13) as well. On the other hand, for $\hbar\omega \ll E_J^*$, the inelastic rate $\Gamma_k^{\rm in}$ vanishes, while the mode shift goes to $\delta\omega_k = -\Delta/2$. One may then compare $\delta\omega_k$ at low frequencies with the mode shifts induced by the two possible boundary conditions — either zero phase variations ($\varphi(x = 0, t) = 0$), imposed by an inductor, or zero current ($\partial_x\varphi(x = 0, t) = 0$), imposed by a capacitor. A shift of half mode spacing is in agreement with the former, indicating a superconducting state.

### D. Exact solution for $z = 1$

An exact solution is available also for $z = 1$. We begin by writing down the Lagrangian for $z = 1$, $\omega_p \to \infty$, and $E_C \to \infty$. Here it is convenient to start from a slightly different geometry, where the small Josephson junction is connected to two waveguides, hence one introduces two fields, $\varphi_r(x)$ and $\varphi_l(x)$:

$$L = \frac{\hbar v}{2\pi} \int_0^l \mathrm{d}x \sum_{\ell=l,r} \left[ \frac{1}{v^2} (\partial_t \varphi_\ell)^2 - (\partial_x \varphi_\ell)^2 \right] + E_J \cos\left(\varphi_l(x=0,t) - \varphi_r(x=0,t)\right). \tag{S25}$$

Note that one recovers the Lagrangian in Eq. (S1) by defining an antisymmetric field, $\varphi = \varphi_l - \varphi_r$; the symmetric field $\varphi_+ = \varphi_l + \varphi_r$ decouples from the impurity. Hence this setup is equivalent to the one considered henceforth, as illustrated in Fig. SF5.

We now proceed by introducing two fermionic fields (again, up to Klein factors [3]),

$$\Psi_\ell(x) = \frac{1}{\sqrt{2\pi b_0}} e^{i\varphi_\ell(x)}, \tag{S26}$$

where $b_0$ is another short distance cutoff. The fermionic fields can again be written in terms of their eigenmodes, $\Psi_\ell(x) = 1/\sqrt{l}\sum_q \Psi_{q\ell} e^{iqx}$, leading to

$$H = \sum_{\ell=l,r} \sum_q \hbar v q \Psi^\dagger_{q\ell} \Psi_{q\ell} - \frac{2\pi b_0 E_J}{2l} \sum_{q,q'} \Psi_{ql} \Psi^\dagger_{q'r} + \text{h.c.} \tag{S27}$$

As for $z = 1/2$, the quadratic form of Eq. (S27) allows for exact calculation of the current-current correlator $K^{\mathcal{R}}(t)$ and hence the AC conductance $\mathcal{G}(\omega)$ in Eq. (S20). Since we are now working in the basis of left and right fields, we should consider two current operators, defined by the time derivative of the total charges in each waveguide,

$$\begin{aligned} Q_\ell &= e \int_0^l \mathrm{d}x \Psi^\dagger_\ell(x) \Psi_\ell(x) = e \sum_q \Psi^\dagger_{q\ell} \Psi_{q\ell}, \\ J_\ell &= \partial_t Q_\ell = -\frac{i}{\hbar} \left[ Q_\ell, H \right] = \pm \frac{ie\pi b_0 E_J}{\hbar l} \sum_{q,q'} \left( \Psi_{q'r} \Psi^\dagger_{ql} - \Psi_{ql} \Psi^\dagger_{q'r} \right) = \pm \frac{eE_J}{\hbar} \sin\left(\varphi_l(x=0,t) - \varphi_r(x=0,t)\right), \end{aligned} \tag{S28}$$

where the plus and minus signs correspond to $J_l$ and $J_r$, respectively. The current operator for the antisymmetric mode is defined by $J_- = J_l - J_r$. A straightforward calculation using the Kubo formula then leads to the backscattered conductance of the antisymmetric mode, $\mathcal{G} = \mathcal{G}_1 \times \frac{4\xi^2}{(1+\xi^2)^2}$, where $\xi = 2\pi b_0 E_J/(4\hbar v)$ and $\mathcal{G}_1 = e^2/(2\pi\hbar)$ is again the conductance of a decoupled waveguide ($E_J = 0$) [4]. The reflection coefficient is defined by $\mathcal{G}/\mathcal{G}_1 = (1-r)/2$; extracting the decay rate and comparing with the perturbative decay rate below the cutoff in Eq. (S10), we identify $\xi = E_J/(\hbar\Gamma_0)$, and therefore

$$r(\omega; z=1) = 1 - \frac{8\left(E_J/(\hbar\Gamma_0)\right)^2}{\left(1 + \left(E_J/(\hbar\Gamma_0)\right)^2\right)^2}. \tag{S29}$$

Note that the exact reflection coefficient depends on neither frequency nor temperature, in agreement with the expected scaling laws. Furthermore, it is real and positive (assuming $E_J \ll \hbar\Gamma_0$), thus no elastic mode shift is predicted by the exact solution. This agrees with Eq. (S13) in the limit $\Gamma_0 \to \infty$, with $E_J/(\hbar\Gamma_0)$ held constant.

### E. Comparison with the experiment

The fitted values $Z^{\mathrm{fit}}$, $E_J^{\mathrm{fit}}$, and $E_C^{\mathrm{fit}}$ in Table ST1, used to produce the theory lines in Fig. 3 of the main text, were obtained as follows. For each device, we allowed a variation in $Z$ around its measured value as well as a variation in $E_C$ near the value given by the measured junction's area plus a realistic capacitance to the leads. For each pair $Z, E_C$, we calculated the elastic mode shift $\delta\omega_k$ and inelastic decay rate $\Gamma_k^{\mathrm{in}}$ using second-order perturbation theory in $E_J/E_C$, Eq. (S9), and normalized both by the yet-unknown $E_J^2$. Comparing both to the experimental data, we obtained two estimates for $E_J$, one from $\delta\omega_k$ and one from $\Gamma_k^{\mathrm{in}}$, denoted by $E_J^{(1)}$ and $E_J^{(2)}$, respectively. The fitted

values, $Z^{\rm fit}$, $E_C^{\rm fit}$, and $E_J^{\rm fit} = E_J^{(2)}$, are those for which the relative error in $E_J$, that is, $\frac{\left|E_J^{(1)} - E_J^{(2)}\right|}{\left(E_J^{(1)} + E_J^{(2)}\right)/2}$, is minimal. A finite, typical temperature of $T = 50$ mK was assumed throughout.


[1] R. Kuzmin, *et al.*, Quantum electrodynamics of a superconductor-insulator phase transition. *Nat. Phys.* **15**, 930 (2019).
[2] M. Abramowitz, I. A. Stegun, *Handbook of Mathematical Functions* (Dover, New York, 1965).
[3] A. O. Gogolin, A. A. Nersesyan, A. M. Tsvelik, *Bosonization and Strongly Correlated Systems* (Cambridge University Press, Cambridge, UK, 2004).
[4] C. L. Kane, M. P. A. Fisher, Transport in a one-channel luttinger liquid. *Phys. Rev. Lett.* **68**, 1220 (1992).
[5] M. Houzet, private communication.
